# Supplementary material for: Error detection using pneumatic logic
Source: arXiv:2401.16500 ancillary file (2024-01-29)

Five replicates of the experiment shown in Figure 4, maintaining each of the 16 possible states for **5 seconds**

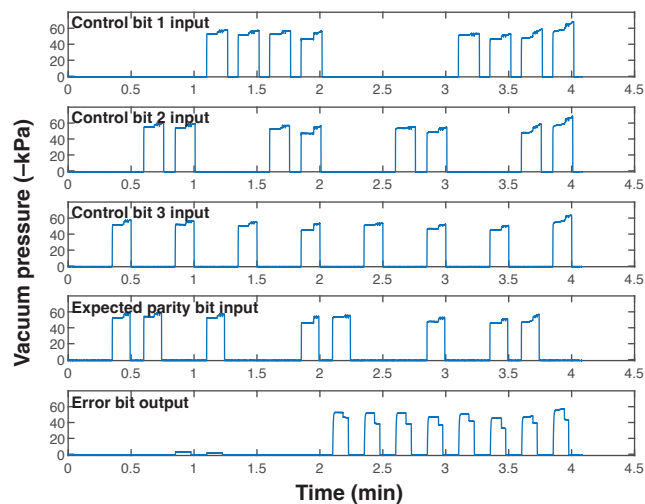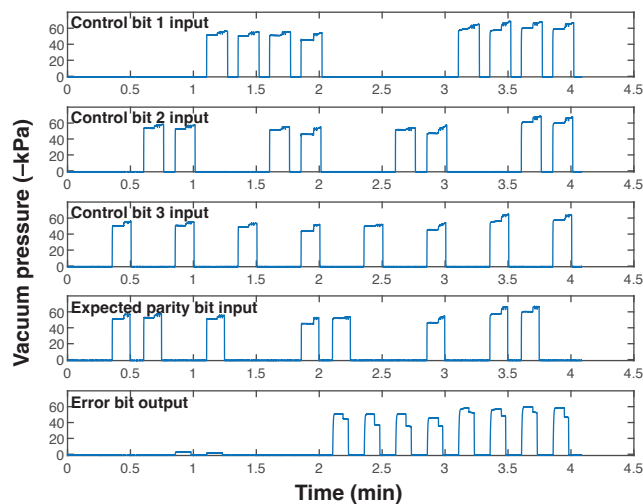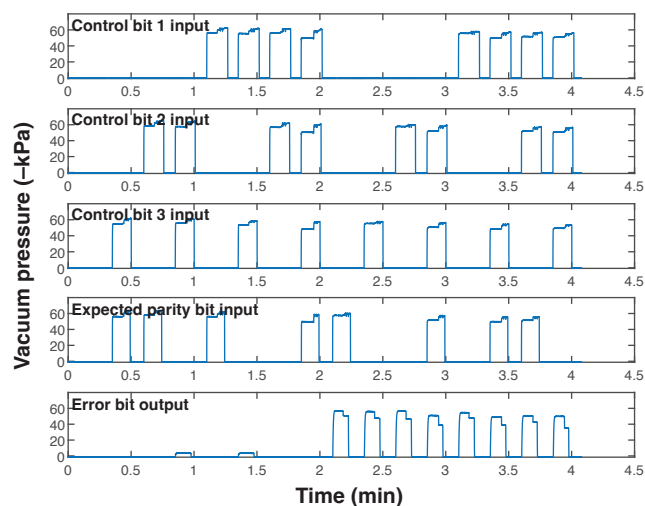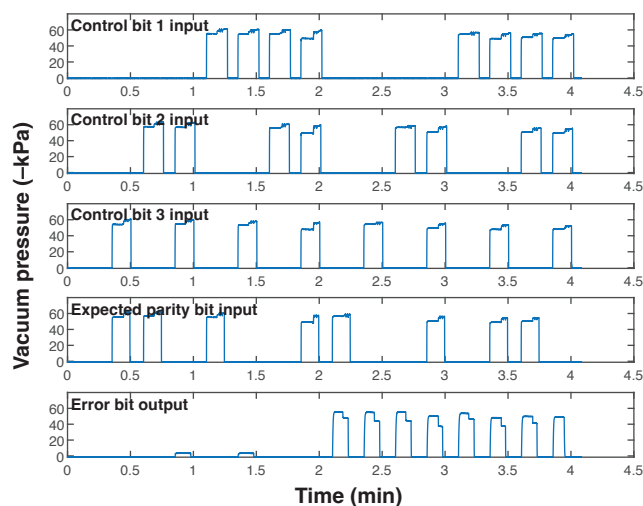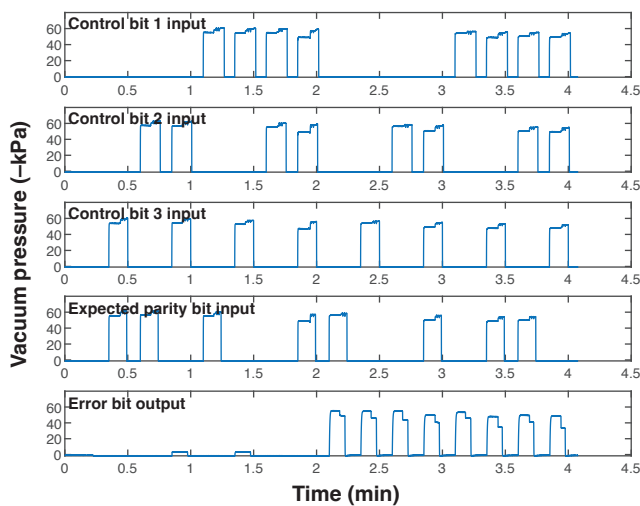

Five replicates of the experiment shown in Figure 4, maintaining each of the 16 possible states for **10 seconds**

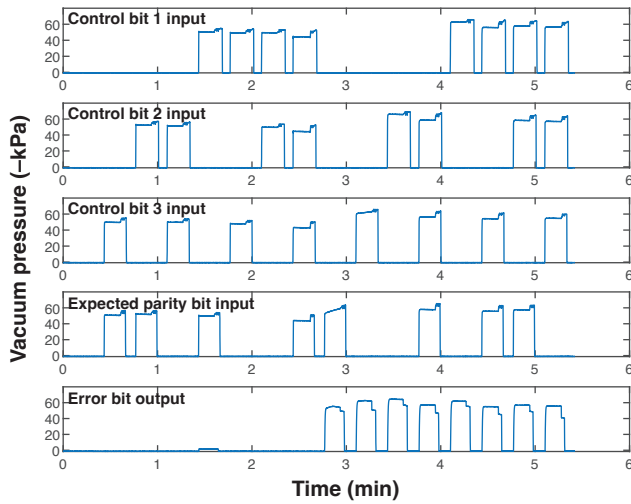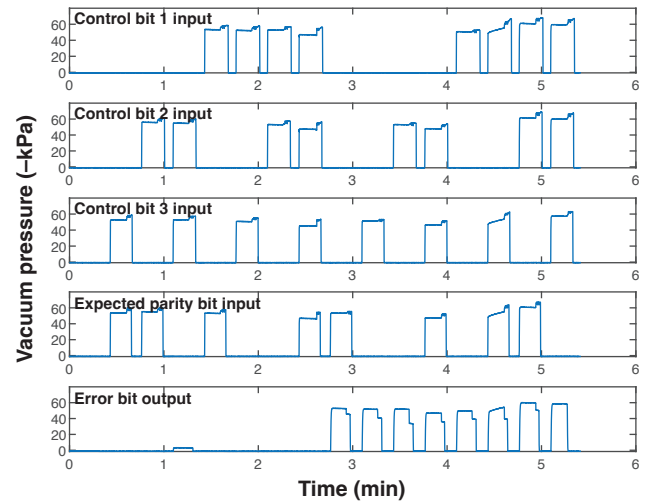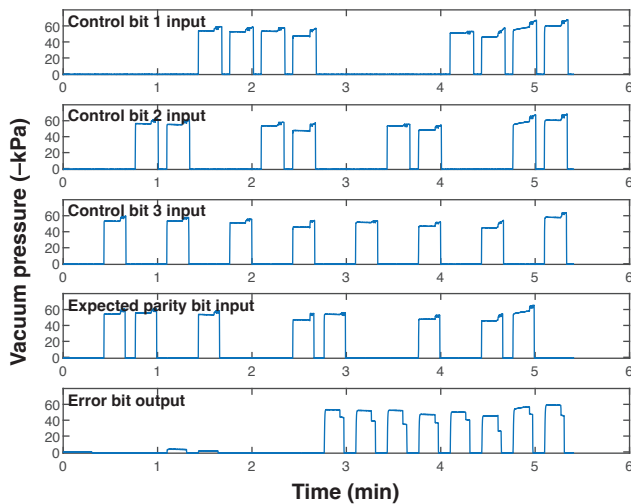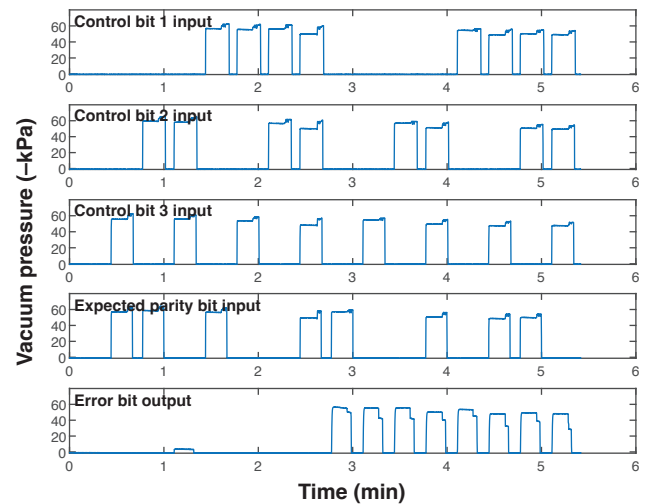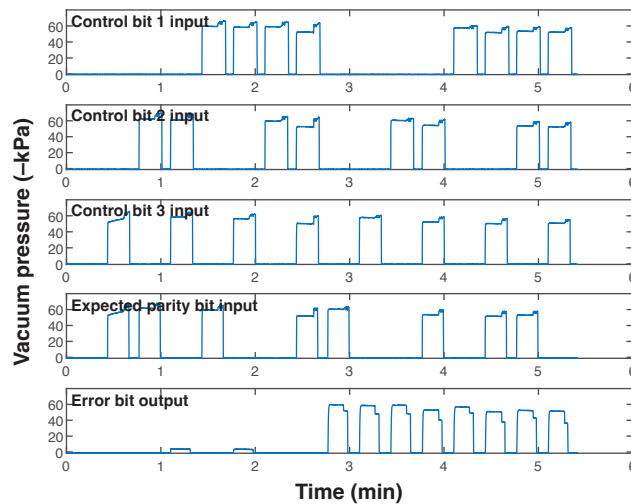

Five replicates of the experiment shown in Figure 4, maintaining each of the 16 possible states for **15 seconds**

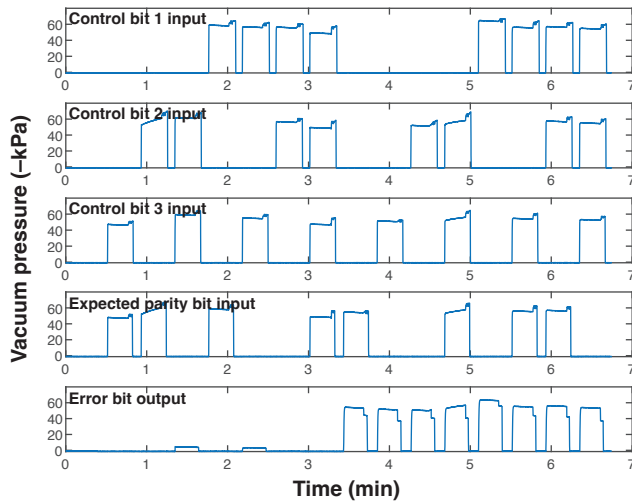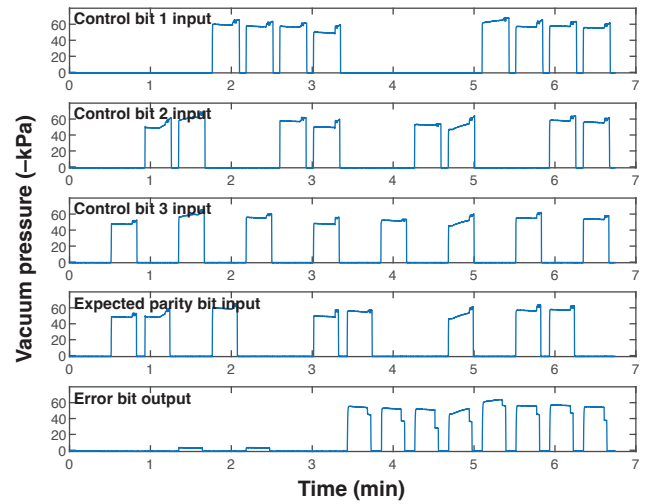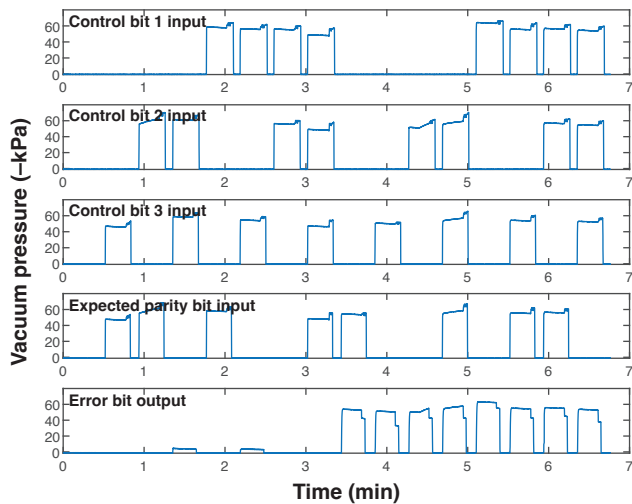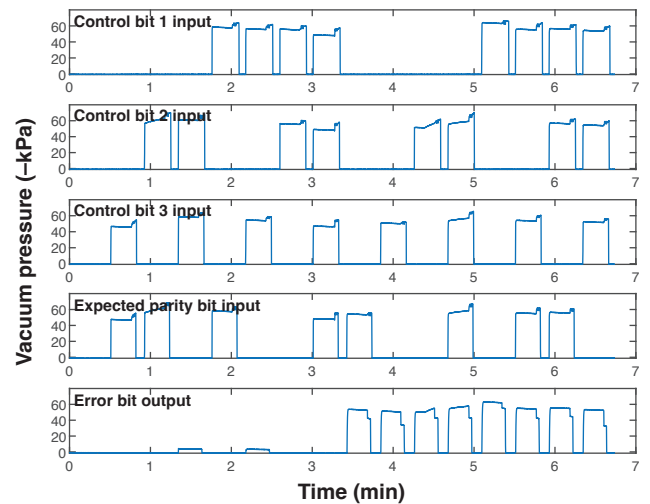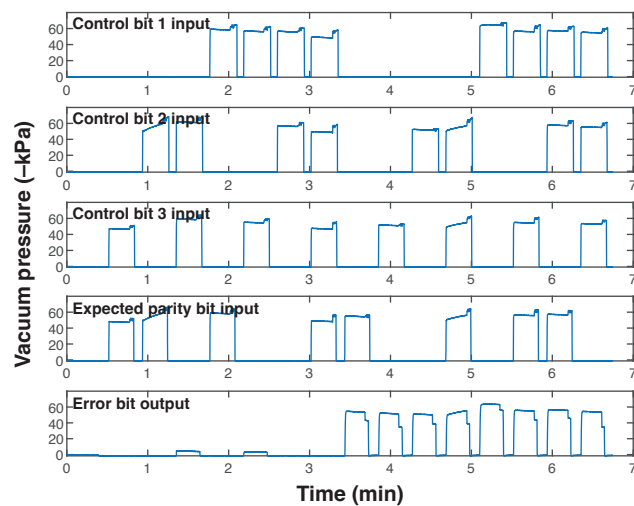

Supplement: Supplementary file 1 [file Figure_4_replicates.pdf]
